# Supplementary material for: Abstraction-Free Control Synthesis to Satisfy Temporal Logic Constraints under Sensor Faults and Attacks
Source: arXiv:2208.10060 source file (2022-08-22)
Supplement: Supplementary file 1 [file appendix.tex]

\section*{Appendix}

This section derives FT-SFCBF. We first define stochastic finite time convergence CBF (SFCBF) under complete information. Then we extend it be under incomplete information. We finally show the fault-tolerant SFCBF (FT-SFCBF).

\begin{definition}[Stochastic Finite Time Convergence CBF under Complete Information]\label{def:FCBF 1}
Consider a dynamical system
\begin{equation*}
    dx_t = (f(x_t)+g(x_t)u_t)dt+\sigma_tdW_t
\end{equation*}
whose solution is denoted as $x(t;x_0)$. Consider a set $\mathcal{C}=\{x:h(x)\geq 0\}$ where $h:\mathbb{R}^n\rightarrow \mathbb{R}$ is locally Lipschitz. A twice continuously differentiable function $B:\mathcal{X}\times[0,\infty)\mapsto\mathbb{R}$ is a stochastic finite time convergence control barrier function if the following conditions hold:
\begin{enumerate}
    \item There exist class $\mathcal{K}_\infty$ functions $\alpha_1$ and $\alpha_2$ such that
    \begin{equation}
        \alpha_1(h(x))\leq B(x)\leq \alpha_2(h(x))
    \end{equation}
    for all $x$.
    \item There exist control input $u$, positive constants $\gamma>0$ and $\rho\in(0,1)$ such that 
    \begin{multline}\label{eq:CLF}
        \frac{\partial B(x)}{\partial x}(f(x)+g(x)u)+\frac{1}{2}tr\left(\sigma_t^\top\frac{\partial^2 B(x)}{\partial x^2}\sigma_t\right)\\
        + \gamma\cdot sgn(B(x)) |B(x)|^\rho\leq 0.
    \end{multline}
\end{enumerate}
\end{definition}

SFCBF provides finite stability in probability guarantee.
\begin{lemma}\label{lemma:SFCBF complete info}
Suppose the system admits an SFCBF $B(x)$. Let $T=\inf\{t:x(t,x_0)\in\mathcal{C}\}$. Then $\mathbb{P}(T<\infty)=1$, i.e., the system reaches $\mathcal{C}$ almost surely. Moreover, the system remains in $\mathcal{C}$ for all $t'\geq T$ almost surely.
\end{lemma}
\begin{proof}
We define a function $B(h(x))$ as $B(h(x))=-h(x)$ if $x\notin Int(\mathcal{C})$ and $B(h(x))=h(x)$ if $x\in\mathcal{C}$. Let $T=\inf\{t:x(t,x_0)\in\mathcal{C}\}$. We then show that $\mathbb{P}(x_t\in\mathcal{C},~\forall t\geq T)=1$ if the system is in $\mathcal{C}$. By the definition of $V$, we have that $B(h(x))=h(x)$. We have that if Eqn. \eqref{eq:CLF} holds, then there must exist some class $\mathcal{K}$ function $\alpha:\mathbb{R}^n\rightarrow\mathbb{R}$ such that
\begin{multline}
        \frac{\partial h(x)}{\partial x}(f(x)+g(x)u)+\frac{1}{2}tr\left(\sigma_t^\top\frac{\partial^2 h(x)}{\partial x^2}\sigma_t\right)\\
        \leq -\gamma|h(x)|^\rho\leq 0\leq \alpha(h(x))
\end{multline}
for all $x\in\mathcal{C}$, indicating that $h(x)$ is a stochastic CBF \cite{clark2019control}. Hence by \cite[Theorem 1]{clark2019control} the system remains in $\mathcal{C}$ for all future time with probability one.

Consider $t\in[0,T)$. In this case if Eqn. \eqref{eq:CLF} holds, we have that
\begin{equation*}
    \frac{\partial B(x)}{\partial x}f(x)+\frac{1}{2}tr\left(\sigma(x)^\top\frac{\partial^2 B(x)}{\partial x^2}\sigma(x)\right) + \gamma\cdot B(x)^\rho\leq 0.
\end{equation*}
Then by Theorem \ref{thm:SCLF}, we have that $\mathbb{P}(T<\infty)=1$, where $T=\inf\{t:h(x(t;x_0))=0\}$ is the stochastic settling time. Hence the system reaches $\mathcal{C}$ almost surely.
\end{proof}

Define 
\begin{equation}
    \Bar{h}_{\varepsilon} = \sup\{h(x):\|x-x'\|_2\leq \varepsilon \text{ for some }x'\in h^{-1}(\{0\})\}
\end{equation}
as the supremum of $h(x)$ for all $x$ belonging to the $\varepsilon$-neighborhood of the boundary of $\mathcal{C}$. We then present the following preliminary result \cite{clark2019control}.
\begin{lemma}[\cite{clark2019control}]\label{lemma:incomplete info safety}
If $\|x_t-\hat{x}_t\|_2\leq \varepsilon$ for all $t$ and $h(\hat{x}_t)>\Bar{h}_\varepsilon$ for all $t$, then $x_t\in\mathcal{C}$ for all $t$.
\end{lemma}

We define $\hat{h}(x)=h(x)-\Bar{h}_\varepsilon$. Provided Lemma \ref{lemma:incomplete info safety}, we are now ready to develop SFCBF under incomplete information setting.
\begin{theorem}
Let $T=\inf\{t:x(t,x_0)\in\mathcal{C}\}$. Suppose there exists a function $B:\mathbb{R}^n\rightarrow\mathbb{R}$, control input $u$, and class $\mathcal{K}$ functions $\alpha_1$ and $\alpha_2$ such that
\begin{subequations}
\begin{align}
    &\alpha_1(\hat{h}(x))\leq B(x)\leq \alpha_2(\hat{h}(x))\\
    &\frac{\partial B}{\partial \hat{x}}(f(x)+g(x)u)+\varepsilon \|\frac{\partial B}{\partial x}K_tc\|_2+\frac{1}{2}tr\left(\sigma_t^\top K_t^\top\frac{\partial^2 B}{\partial \hat{x}^2}K_t\sigma_t\right)\nonumber\\
    &\quad\quad\quad+ \gamma\cdot sgn(\hat{h}(\hat{x}_t))|\hat{h}(\hat{x}_t)|^\rho\leq 0\label{eq:SFCBF incomplete info}
\end{align}
\end{subequations}
then $\mathbb{P}(T<\infty)\geq 1-\zeta$, i.e., the system reaches $\mathcal{C}$ with probability at least $1-\zeta$.
\end{theorem}
\begin{proof}
Since we use EKF for state estimation, we have that
\begin{equation}
    d\hat{x}_t=f(\hat{x}_t) + g(\hat{x}_t)u_td_t + K_t(dy_t-c\hat{x}_tdt),
\end{equation}
where $K_t=P_tc^\top R_t^{-1}$ is the Kalman gain, $R_t=\nu_t^\top\nu_t$, and $P_t$ is the solution to the following Riccati equation:
\begin{equation}
    \frac{dP}{dt}=A_tP_t+P_tA_t^\top +Q_t-P_tc^\top R_t^{-1}cP_t,
\end{equation}
with $A_t=\frac{\partial(f(\hat{x}_t) + g(\hat{x}_t)u_t)}{\partial x}$ and $Q_t=\sigma_t^\top\sigma_t$. Given the output dynamics of $y_t$, we have that
\begin{align*}
    d\hat{x}_t&=(f(\hat{x}_t) + g(\hat{x}_t)u_t)d_t + K_t(cx_tdt+\nu_tdV_t-c\hat{x}_tdt)\\
    &=(f(\hat{x}_t) + g(\hat{x}_t)u_t + K_tc(x_t-\hat{x}_t))dt + K_t\nu_tdV_t.
\end{align*}
Let $B_t=B(\hat{x}_t)$. We then have that
\begin{multline}
    dB_t = \bigg(\frac{\partial B}{\partial \hat{x}}\left(f(\hat{x}_t) + g(\hat{x}_t)u_t + K_tc(x_t-\hat{x}_t)\right)\\
    +\frac{1}{2}tr\left(\nu_t^\top K_t^\top \frac{\partial^2 B}{\partial \hat{x}}K_t\nu_t\right)\bigg)dt + \frac{\partial B}{\partial \hat{x}}K_t\nu_tdV_t.
\end{multline}
When $\|x_t-\hat{x}_t\|_2\leq \varepsilon$ holds, then 
\begin{equation*}
    \frac{\partial B}{\partial \hat{x}}K_tc(x_t-\hat{x}_t)\leq  \left\|\frac{\partial B}{\partial \hat{x}}K_tc\right\|_2\|x_t-\hat{x}_t\|_2\leq \varepsilon\left\|\frac{\partial B}{\partial \hat{x}}K_tc\right\|_2.
\end{equation*}
When Eqn. \eqref{eq:SFCBF incomplete info} holds, we thus have that
\begin{align*}
    &\frac{\partial B}{\partial \hat{x}}\left(f(\hat{x}_t) + g(\hat{x}_t)u_t + K_tc(x_t-\hat{x}_t)\right)\\
    &\quad\quad\quad+\frac{1}{2}tr\left(\nu_t^\top K_t^\top \frac{\partial^2 B}{\partial \hat{x}^2}K_t\nu_t\right)\\
    \leq&\frac{\partial B}{\partial \hat{x}}\left(f(\hat{x}_t) + g(\hat{x}_t)u_t\right) + \varepsilon\left\|\frac{\partial B}{\partial \hat{x}}K_tc\right\|_2\\
    &\quad\quad\quad+\frac{1}{2}tr\left(\nu_t^\top K_t^\top \frac{\partial^2 B}{\partial \hat{x}^2}K_t\nu_t\right)\\
    \leq & -\gamma\cdot sgn(\hat{h}(\hat{x}_t))|\hat{h}(\hat{x}_t)|^\rho.
\end{align*}
Finally, according to Lemma \ref{lemma:SFCBF complete info}, we have that there exists some time $T=\inf\{t:x(t;x_0)\in\mathcal{C}\}$ is finite with probability $\mathbb{P}(T<\infty)\geq 1-\zeta$.
\end{proof}

We are now ready to present FT-SFCBF as follows.
\begin{theorem}\label{thm:FT-SFCBF}
Let $\Bar{h}_{\varepsilon_i} = \sup\{h(x):\|x-x'\|_2\leq \varepsilon_i \text{ for some }x'\in h^{-1}(\{0\})\}$ and $\hat{h}_i(x)=h(x)-\Bar{h}_{\varepsilon_i}$. Let $T=\inf\{t:x(t;x_0)\in\mathcal{C}\}$. Suppose $\varepsilon_1,\ldots,\varepsilon_m$ and $\theta_{ij}$ are chosen such that
\begin{enumerate}
    \item There exists $\varrho>0$ such that for any $X_t'\subseteq X_t(\varrho)$ satisfying $\|\hat{x}_{t,i}-\hat{x}_{t,j}\|\leq \theta_{ij}$ for all $i,j\in X_t'$ there exists $u$ satisfying
    \begin{equation}
        \Lambda_i(\hat{x}_{t,i})u>0,~\forall i\in X_t'
    \end{equation}
    where $\Lambda_i(\hat{x}_{t,i})=\frac{\partial h_i}{\partial x}(\hat{x}_{t,i})g(\hat{x}_{t,i})$, $X_t(\varrho)=\{i:\hat{h}_i(\hat{x}_{t,i})<\varrho\}$.
    \item For each $i$, when $r=r_i$,
    \begin{equation}
        \mathbb{P}(\|\hat{x}_{t,i}-\hat{x}_{t,i,j}\|_2\leq\theta_{ij}/2,~\forall j, \|\hat{x}_{t,i}-x_t\|_2\leq \varepsilon_i,~\forall t)\geq 1-\zeta,
    \end{equation}
    then $\mathbb{P}(T<\infty)\geq 1-\zeta$.
\end{enumerate}
\end{theorem}
Functions $h_1,\ldots,h_m$ satisfying conditions 1) and 2) in Theorem \ref{thm:FT-SFCBF} are FT-SFCBFs.
